# Supplementary material for: Design the Feedback, Not Just the Reward: Environments for Open-Ended Reinforcement Learning
Source: arXiv:2608.27906 source file (2026-10-29)
Supplement: Supplementary file 1 [file appendix.tex]

% !TeX root = ../main.tex

\section{Data Construction Details}
\label{app:data_construction}


\section{Additional Details on Hierarchical Reward}
\label{app:reward_detail}

\section{Details of Experimental Setup}
\label{app:exp_details}
